# Supplementary material for: An Empirical Study on Benchmarks of Artificial Software Vulnerabilities
Source: arXiv:2003.09561 source file (2020-03-21)
Supplement: Supplementary file 1 [file A-appendix.tex]

%%
%% If your work has an appendix, this is the place to put it.
\appendix

\section{Real-World Vulnerabilities of CVEs}\label{apendix:cve_ids}

\begin{table}[htbp]
\tiny
\centering
\caption{The real-world vulnerabilities with CVE-IDs in the dataset.}
\label{tab:CVE-ID}
\begin{tabular*}{\linewidth}{p{1cm}|p{1.2cm}|p{1.2cm}|p{1.2cm}|p{1.2cm}|p{1.2cm}|p{1cm}}
\hline
\multicolumn{1}{c|}{\textbf{Type}} & \textbf{2004-2006}                                                                                                                                                                 & \textbf{2007-2009}                                                                                                                                   & \textbf{2010-2012}                                                                                                                                   & \multicolumn{1}{c|}{\textbf{2013-2015}}                                                                                         & \multicolumn{1}{c|}{\textbf{2016-2018}}                                                                                         & \multicolumn{1}{l}{\textbf{Sum}} \\ \hline
\textbf{Stack Overflow}            & \multicolumn{1}{l|}{\begin{tabular}[c]{@{}l@{}}CVE-2004-0597 CVE-2004-1120\\ CVE-2004-1257 CVE-2004-1262\\ CVE-2004-1265 CVE-2004-1287\\ CVE-2004-1288 CVE-2004-1290\end{tabular}} & \multicolumn{1}{l|}{\begin{tabular}[c]{@{}l@{}}CVE-2007-1825 CVE-2007-2683\\ CVE-2007-6454 CVE-2009-2286\\ CVE-2009-3050 CVE-2009-5018\end{tabular}} & \multicolumn{1}{l|}{\begin{tabular}[c]{@{}l@{}}CVE-2010-1147 CVE-2010-2891\\ CVE-2010-4221 CVE-2010-4259\\ CVE-2011-1071 CVE-2012-4409\end{tabular}} & \begin{tabular}[c]{@{}l@{}}CVE-2013-0222 CVE-2013-0223\\ CVE-2013-0722 CVE-2014-8322\\ CVE-2015-5895 CVE-2015-7547\end{tabular} & \begin{tabular}[c]{@{}l@{}}CVE-2016-10095 CVE-2016-2233\\ CVE-2016-2563 CVE-2017-9147\\ CVE-2017-9160\end{tabular}              & 31                            \\ \hline
\textbf{Heap Overflow}             & \multicolumn{1}{l|}{\begin{tabular}[c]{@{}l@{}}CVE-2005-1275 CVE-2006-0539\\ CVE-2006-3582 CVE-2006-4018\end{tabular}}                                                             & \multicolumn{1}{l|}{\begin{tabular}[c]{@{}l@{}}CVE-2007-1286 CVE-2008-5904\\ CVE-2008-1887\end{tabular}}                                             & \multicolumn{1}{l|}{\begin{tabular}[c]{@{}l@{}}CVE-2010-1159 CVE-2010-2089\\ CVE-2012-4412\end{tabular}}                                             & \begin{tabular}[c]{@{}l@{}}CVE-2013-4243 CVE-2013-7226\\ CVE-2015-7805\end{tabular}                                             & \begin{tabular}[c]{@{}l@{}}CVE-2017-9170 CVE-2017-9171\\ CVE-2017-9172 CVE-2017-9173\\ CVE-2017-9189 CVE-2017-9191\end{tabular} & 19                               \\ \hline
\textbf{Integer Overflow}          & \multicolumn{1}{l|}{\begin{tabular}[c]{@{}l@{}}CVE-2004-0597 CVE-2004-0990\\ CVE-2006-2025 CVE-2006-2971\end{tabular}}                                                             & \multicolumn{1}{l|}{\begin{tabular}[c]{@{}l@{}}CVE-2007-1777 CVE-2008-2315\\ CVE-2009-4880\end{tabular}}                                             & \multicolumn{1}{l|}{\begin{tabular}[c]{@{}l@{}}CVE-2010-4409 CVE-2011-1092\\ CVE-2011-1137\end{tabular}}                                             & CVE-2014-7185 CVE-2013-7226                                                                                                     & CVE-2016-9819 CVE-2017-7599                                                                                                     & 14                               \\ \hline
\textbf{NULL Pointer Dereference}  & ---                                                                                                                                                                                & \multicolumn{1}{l|}{CVE-2007-3473}                                                                                                                   & \multicolumn{1}{l|}{CVE-2010-2481 CVE-2010-2482}                                                                                                     & \multicolumn{1}{c|}{---}                                                                                                        & CVE-2016-7445 CVE-2017-5980                                                                                                     & 5                                \\ \hline
\textbf{Format String}             & ---                                                                                                                                                                                & ---                                                                                                                                                  & \multicolumn{1}{l|}{CVE-2012-0809}                                                                                                                   & \begin{tabular}[c]{@{}l@{}}CVE-2013-2131 CVE-2013-4474\\ CVE-2015-8617\end{tabular}                                             & \multicolumn{1}{c|}{---}                                                                                                        & 4                                \\ \hline
\textbf{Use After Free}            & ---                                                                                                                                                                                & ---                                                                                                                                                  & ---                                                                                                                                                  &  \multicolumn{1}{l|}{CVE-2015-3890}                                                                                                                   &  \multicolumn{1}{l|}{CVE-2017-9182}                                                                                                                   & 2                                \\ \hline
\textbf{Invalid Access}            & ---                                                                                                                                                                                & ---                                                                                                                                                  & ---                                                                                                                                                  & \multicolumn{1}{c|}{---}                                                                                                        & CVE-2017-9174 CVE-2017-9177                                                                                                     & 2                                \\ \hline
\textbf{Invalid Free}              & ---                                                                                                                                                                                & \multicolumn{1}{l|}{CVE-2008-1767}                                                                                                                   & ---                                                                                                                                                  & \multicolumn{1}{c|}{---}                                                                                                        &  \multicolumn{1}{l|}{CVE-2017-9190}                                                                                                                  & 2                                \\ \hline
\textbf{Other}                     & ---                                                                                                                                                                                & ---                                                                                                                                                  & ---                                                                                                                                                  &  \multicolumn{1}{l|}{CVE-2014-6277}                                                                                                                   & \multicolumn{1}{c|}{---}                                                                                                        & 1                                \\ \hline
\textbf{Sum}                       & 16                                                                                                                                                                                 & 14                                                                                                                                                   & 15                                                                                                                                                   & \multicolumn{1}{c|}{16}                                                                                                         & \multicolumn{1}{c|}{19}                                                                                                         & 80                               \\ \hline
\end{tabular*}
\end{table}

% \subsection{Part One}

% Lorem ipsum dolor sit amet, consectetur adipiscing elit. Morbi
% malesuada, quam in pulvinar varius, metus nunc fermentum urna, id
% sollicitudin purus odio sit amet enim. Aliquam ullamcorper eu ipsum
% vel mollis. Curabitur quis dictum nisl. Phasellus vel semper risus, et
% lacinia dolor. Integer ultricies commodo sem nec semper.

% \subsection{Part Two}

% Etiam commodo feugiat nisl pulvinar pellentesque. Etiam auctor sodales
% ligula, non varius nibh pulvinar semper. Suspendisse nec lectus non
% ipsum convallis congue hendrerit vitae sapien. Donec at laoreet
% eros. Vivamus non purus placerat, scelerisque diam eu, cursus
% ante. Etiam aliquam tortor auctor efficitur mattis.

% \section{Online Resources}

% Nam id fermentum dui. Suspendisse sagittis tortor a nulla mollis, in
% pulvinar ex pretium. Sed interdum orci quis metus euismod, et sagittis
% enim maximus. Vestibulum gravida massa ut felis suscipit
% congue. Quisque mattis elit a risus ultrices commodo venenatis eget
% dui. Etiam sagittis eleifend elementum.

% Nam interdum magna at lectus dignissim, ac dignissim lorem
% rhoncus. Maecenas eu arcu ac neque placerat aliquam. Nunc pulvinar
% massa et mattis lacinia.
